# Supplementary material for: Statistical Inference for High-Dimensional Matrix-Variate Factor Model
Source: arXiv:2001.01890 source file (2022-10-19)
Supplement: Supplementary file 1 [file appendix-more-results.tex]

\section{More Simulation Results}  \label{sec:more-results}

In this section, we present the more simulation results for Setting (I) and (III).
Results are similar to those for Setting (II) presented at the main text.
For both latent dimension estimation and convergence results, $\alpha$-PCA consistently converges faster with lower variance and estimates more accurately than AC-PCA over all chosen settings.
Thus it is implied that $\alpha$-PCA has significant advantages over AC-PCA when $\bF_t$ and $\bE_t$ are uncorrelated or weakly correlated across rows and columns or time.

\subsection{Uncorrelated across time, rows, and columns}

This section presents results for Setting (I) where $\bE_t$ are uncorrelated across time, rows, and columns.
The entries of both $\bF_t$ and $\bE_t$ are uncorrelated across time, rows and columns. Specifically, we simulate temporally independent $\bF_t \sim \calM \calN_{3 \times 3} \left( \bzero, \bI, \bI \right)$ and $\bE_t \sim \calM \calN_{p \times q} \left( \bzero, \bI, \bI \right)$.

Table \ref{table:estim_k_I} and \ref{table:mean_sd_I} presents the frequencies of estimated $(\hat k, \hat r)$ pairs and means and standard deviations of $D(\hat{\bR}, \bR)$),$D(\hat{\bC}, \bC)$), respectively, for Setting (I).

%table estimated dimensions (Wang, Chen)
\begin{table} [htpb!]
    \centering
    \resizebox{\textwidth}{!}{
    \begin{tabular}{c| c c c c |c c c c | c c c c } \hline
	\multicolumn{5}{c}{$p,q = 20,20$} & \multicolumn{4}{c}{$p,q = 100,20$} & \multicolumn{4}{c}{$p,q = 100,100$}\\ \hline
	($\hat{k},\hat{r}$)  & $T=.5pq$ & $T=pq$& $T=1.5pq$& $T=2pq$ & $T=.5pq$ & $T=pq$& $T=1.5pq$& $T=2pq$ & $T=.5pq$ & $T=pq$& $T=1.5pq$& $T=2pq$\\ \hline
	($2,3$) & .05 &  .085 & .035 & .035& 0    & 0   & 0    & 0 & 0 & 0 & 0 &0\\
    \rowcolor[HTML]{EFEFEF}  & .025 & .005 & .005 & .015  & 0 & 0 & 0 & 0 & 0 & 0 & 0 &0\\ \hline
	($3,2$) & .05 &  .03 & .01   & .045& .025 & .015&.015  & .02 &  0 & 0 &0 &0\\
    \rowcolor[HTML]{EFEFEF} & .01 & .015 & 0 & .01 & .005 & .005 & 0 & 0 & 0 & 0 &0 &0\\ \hline
	($3,3$) & .845 &  .835 & .92 & .895& .975 & .975& .98  & .975 & 1 &1 & 1 & 1\\
    \rowcolor[HTML]{EFEFEF}  & .955 &  .975 & .995 & .975 & .995 & .995 & 1 & 1 & 1 &1 &1 & 1\\ \hline
	other  & .055   & .05 & .03 & .01   & 0    & .01   & .005    & .005 & 0 & 0 & 0 & 0\\
    \rowcolor[HTML]{EFEFEF}  & .01 & .005 & 0 & 0 & 0 & 0 & 0 & 0 & 0 & 0 & 0 & 0\\ \hline
	\end{tabular}}%
    \caption{Table of frequencies of estimated ($\hat{k}, \hat{r}$) pairs estimated by $\alpha$-PCA (highlighted rows) and AC-PCA (not highlighted rows) under Setting I. The truth is $(3,3)$.}  \label{table:estim_k_I}
\end{table}

\begin{table}[htpb!]
\centering
\resizebox{\linewidth}{!}{\begin{tabular}{c c c c c c c c c} \hline
& \multicolumn{2}{c}{$T = 0.5pq$} & \multicolumn{2}{c}{$T = pq$} & \multicolumn{2}{c}{$T = 1.5pq$} & \multicolumn{2}{c}{$T = 2pq$} \\ \hline
$(p,q)$  & D($\hat{\bR},\bR$) &  D($\hat{\bC},\bC$) & D($\hat{\bR},\bR$) &  D($\hat{\bC},\bC$) & D($\hat{\bR},\bR$) &  D($\hat{\bC},\bC$) & D($\hat{\bR},\bR$) &  D($\hat{\bC},\bC$)\\ \hline
\rowcolor[HTML]{EFEFEF}($20,20$) & .40(.08) & .40(.09)  & .28(.07) & .29(.07) & .23(.05) & .23(.05) & .20(.05) & .20(.04) \\
& 1.11(.24) & 1.12(.31)  & 1.11(.27) & 1.11(.26) & 1.07(.23) & 1.10(.22) & 1.08(.27) & 1.09(.22) \\
\rowcolor[HTML]{EFEFEF}($100,20$) & .14(.01) & .08(.02) & .10(.01) & .05(.01) & .08(.01) & .04(.01) & .07(.01) & .04(.01) \\
& .80(.07) & .45(.10) & .80(.07) & .45(.10) & .80(.07) & .45(.10) & .80(.07) & .44(.09) \\
\rowcolor[HTML]{EFEFEF}($100,100$) & .03(.002) & .03(.002) & .02(.002) & .02(.002) & .02(.001) & .02(.001) & .01(.001) & .01(.001)  \\
& .34(.02) & .34(.03) & .34(.03) & .33(.03) & .34(02) & .33(.02) & .34(.03) & .33(.03)  \\ \hline
\end{tabular}}
\caption{Means and standard deviations in parentheses of $D(\hat{\bR}, \bR)$),$D(\hat{\bC}, \bC)$) estimated by $\alpha$-PCA (highlighted) and AC-PCA (not highlighted rows) under Setting I. All values multiplied by 10 and rounded for ease of presentation.} \label{table:mean_sd_I}
\end{table}

Figure \ref{fig:space_dist_ratio_I_III} (a) shows the box plots of the ratios between space distances $\calD(\hat \bR, \bR)$, $\calD(\hat \bC, \bC)$ of the two methods under Setting (I).
The estimation error of $\alpha$-PCA is much smaller than AC-PCA.

Figure \ref{fig:F_norm_I_III} (a) presents the box plots of $\ell_2$ norm of distance between $\hat\bF_t$ estimated by $\alpha$-PCA and transformed true $\bF_t$, which shows the convergence of estimated factors under Setting (I).

% boxplot space distance ratio (Wang, Chen)
\begin{figure}
\centering
\begin{subfigure}[b]{\textwidth}
\centering
\caption{Setting (I). }
\includegraphics[width=\linewidth,height=\textheight,keepaspectratio=true]{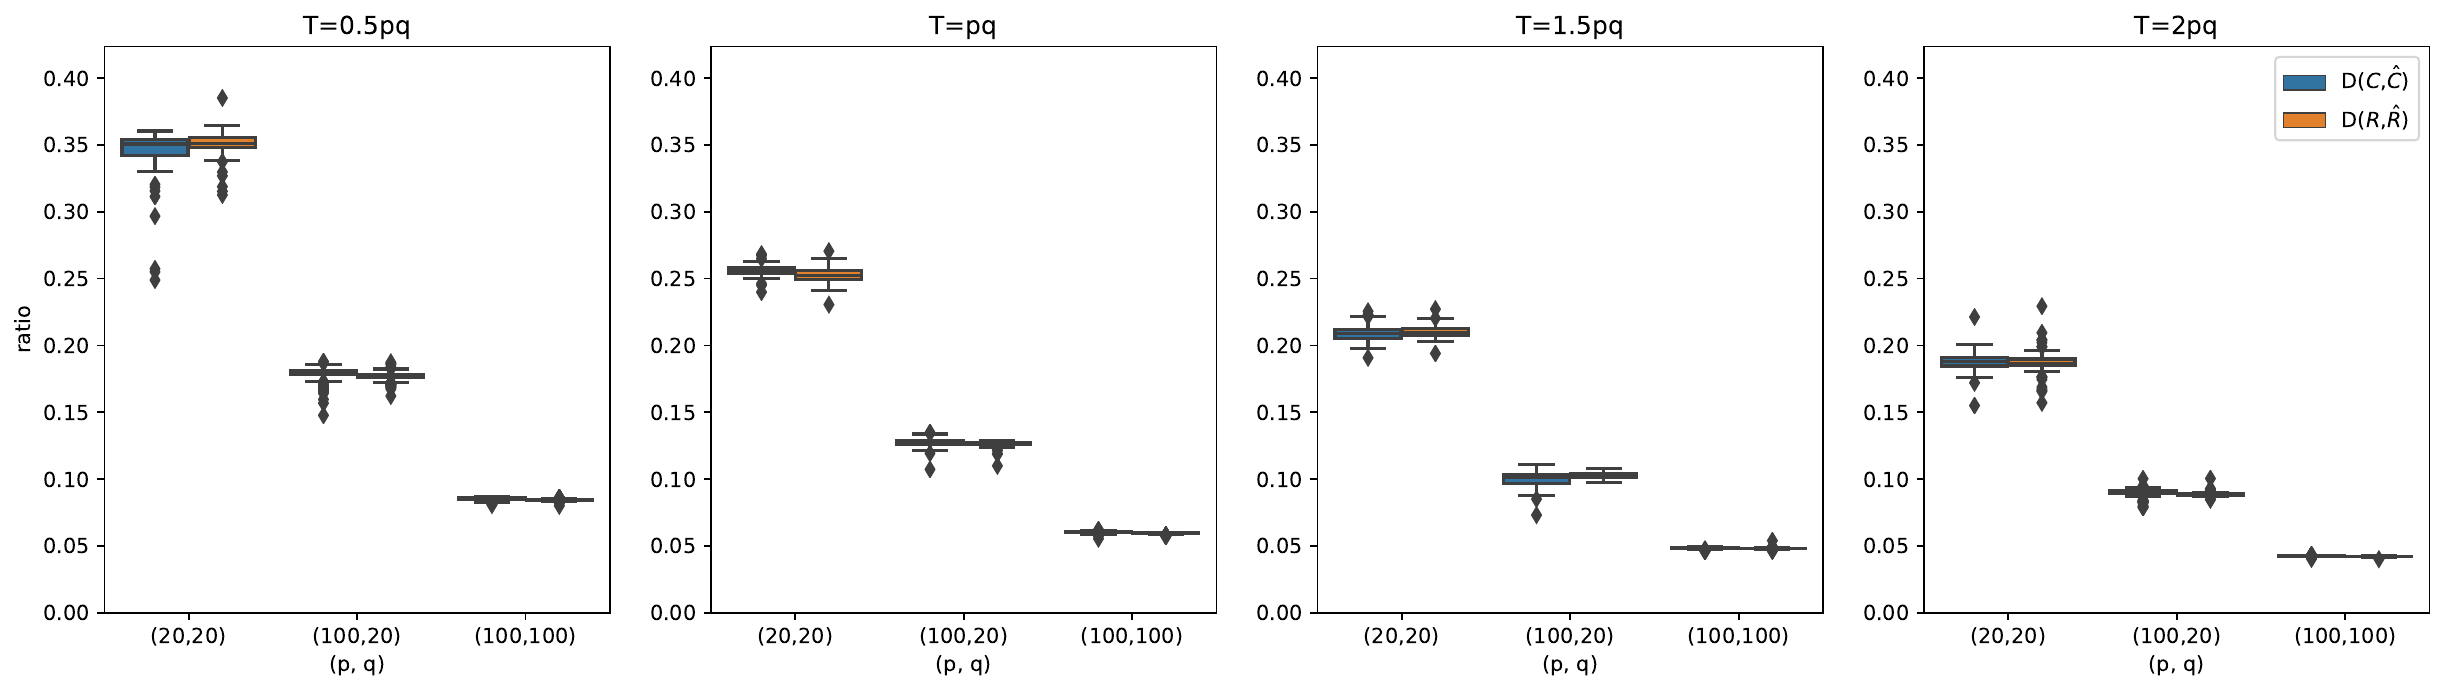}
\end{subfigure}
\hfill
\begin{subfigure}[b]{\textwidth}
\centering
\caption{Setting (III). }
\includegraphics[width=\linewidth,height=\textheight,keepaspectratio=true]{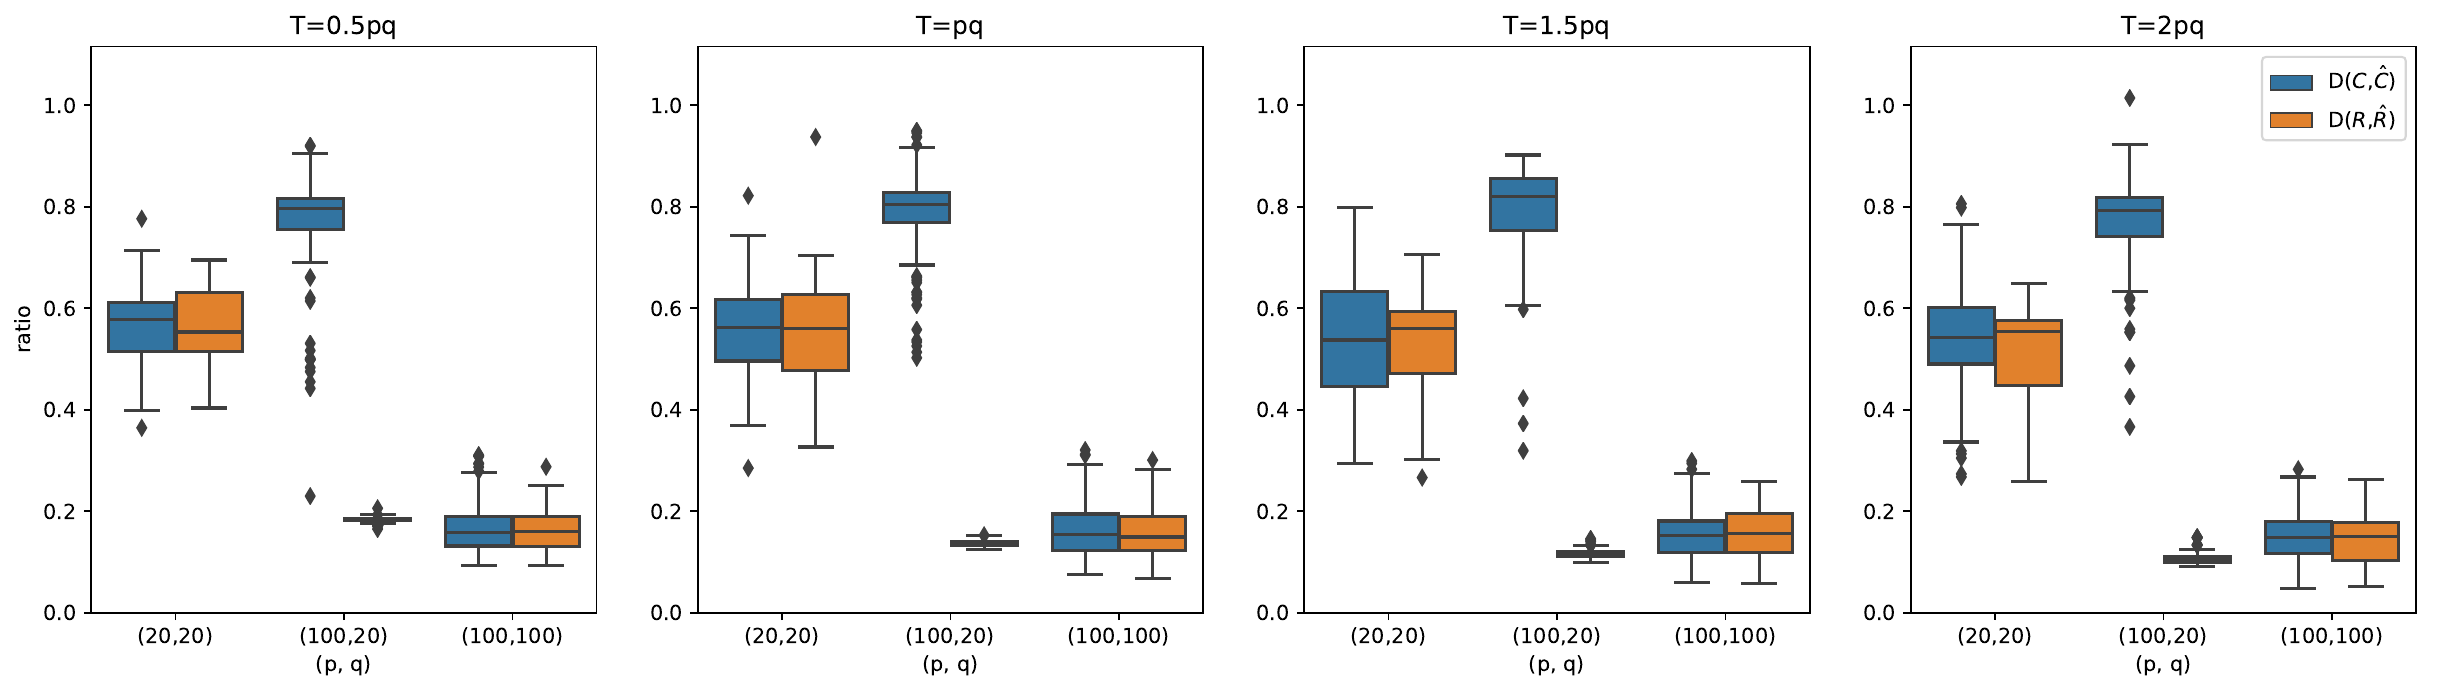}
\end{subfigure}
\caption{Box plots of ratios of space distances between $\alpha$-PCA and AC-PCA estimators.
(a) is under Setting I; (b) is under Setting III. The estimation errors of $\alpha$-PCA is much smaller than AC-PCA}.
\label{fig:space_dist_ratio_I_III}
\end{figure}

%boxplot F norm
\begin{figure}[htpb!]
\centering
\begin{subfigure}[b]{\textwidth}
\centering
\caption{Setting (I).}
\includegraphics[width=\linewidth,height=\textheight,keepaspectratio=true]{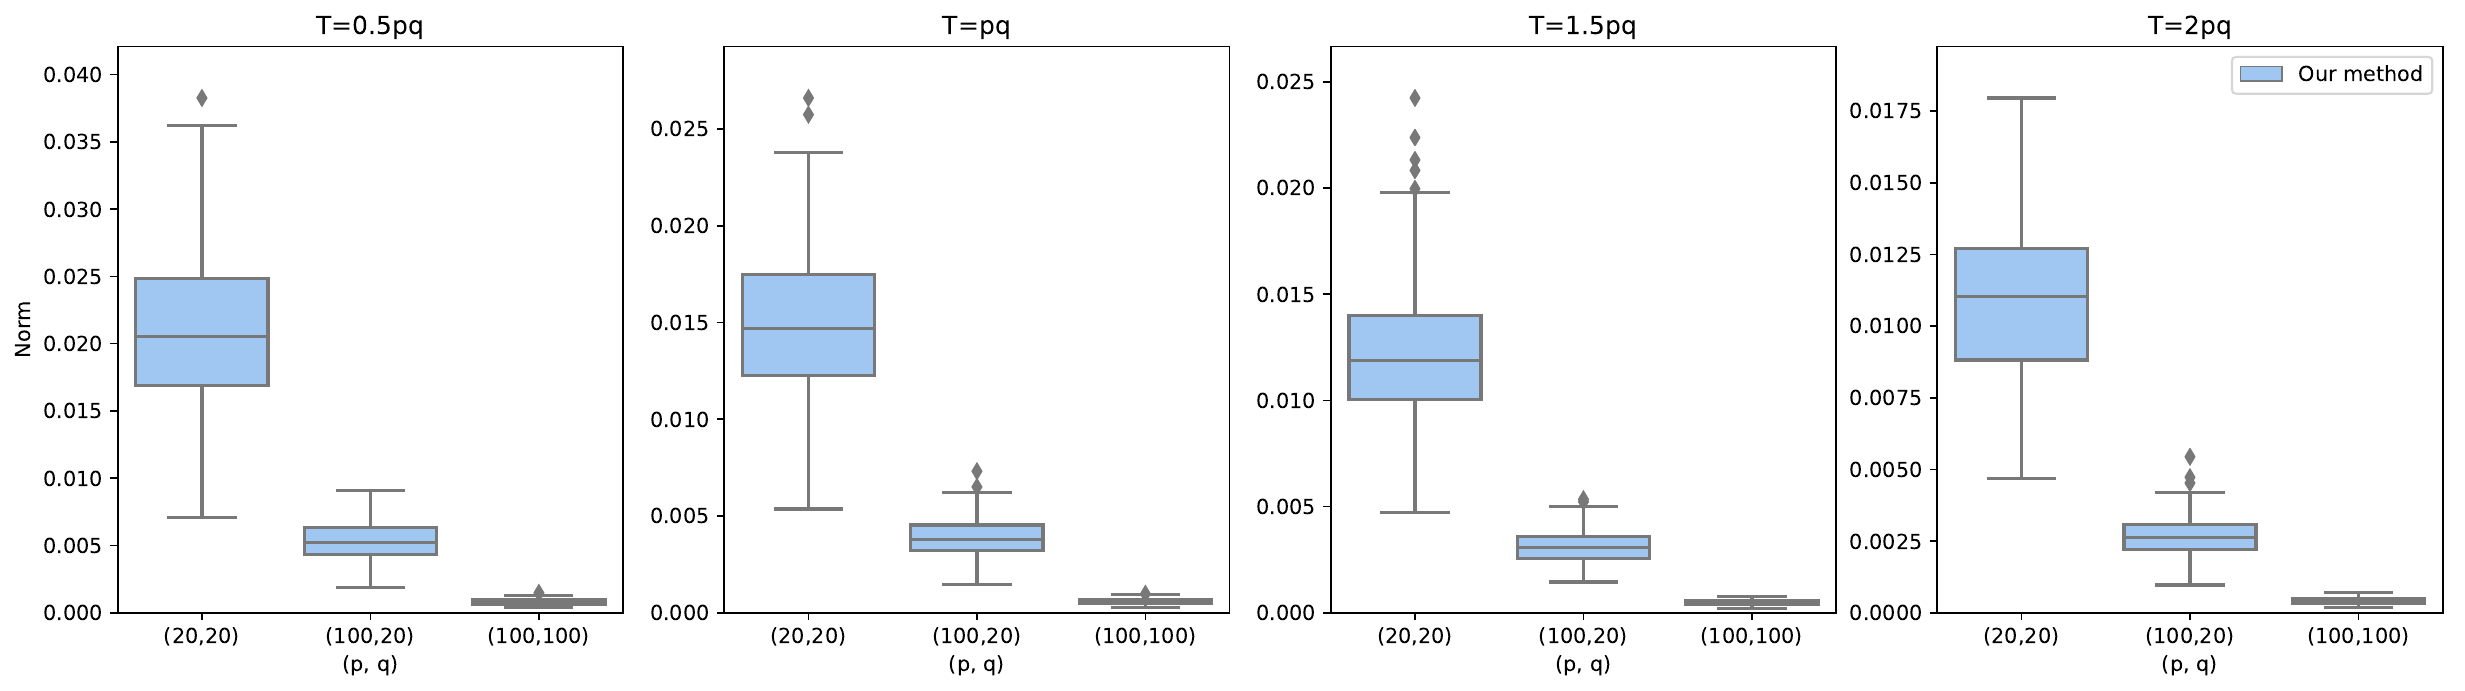}
\end{subfigure}
\hfill
\begin{subfigure}[b]{\textwidth}
\centering
\caption{Setting (III).}
\includegraphics[width=\linewidth,height=\textheight,keepaspectratio=true]{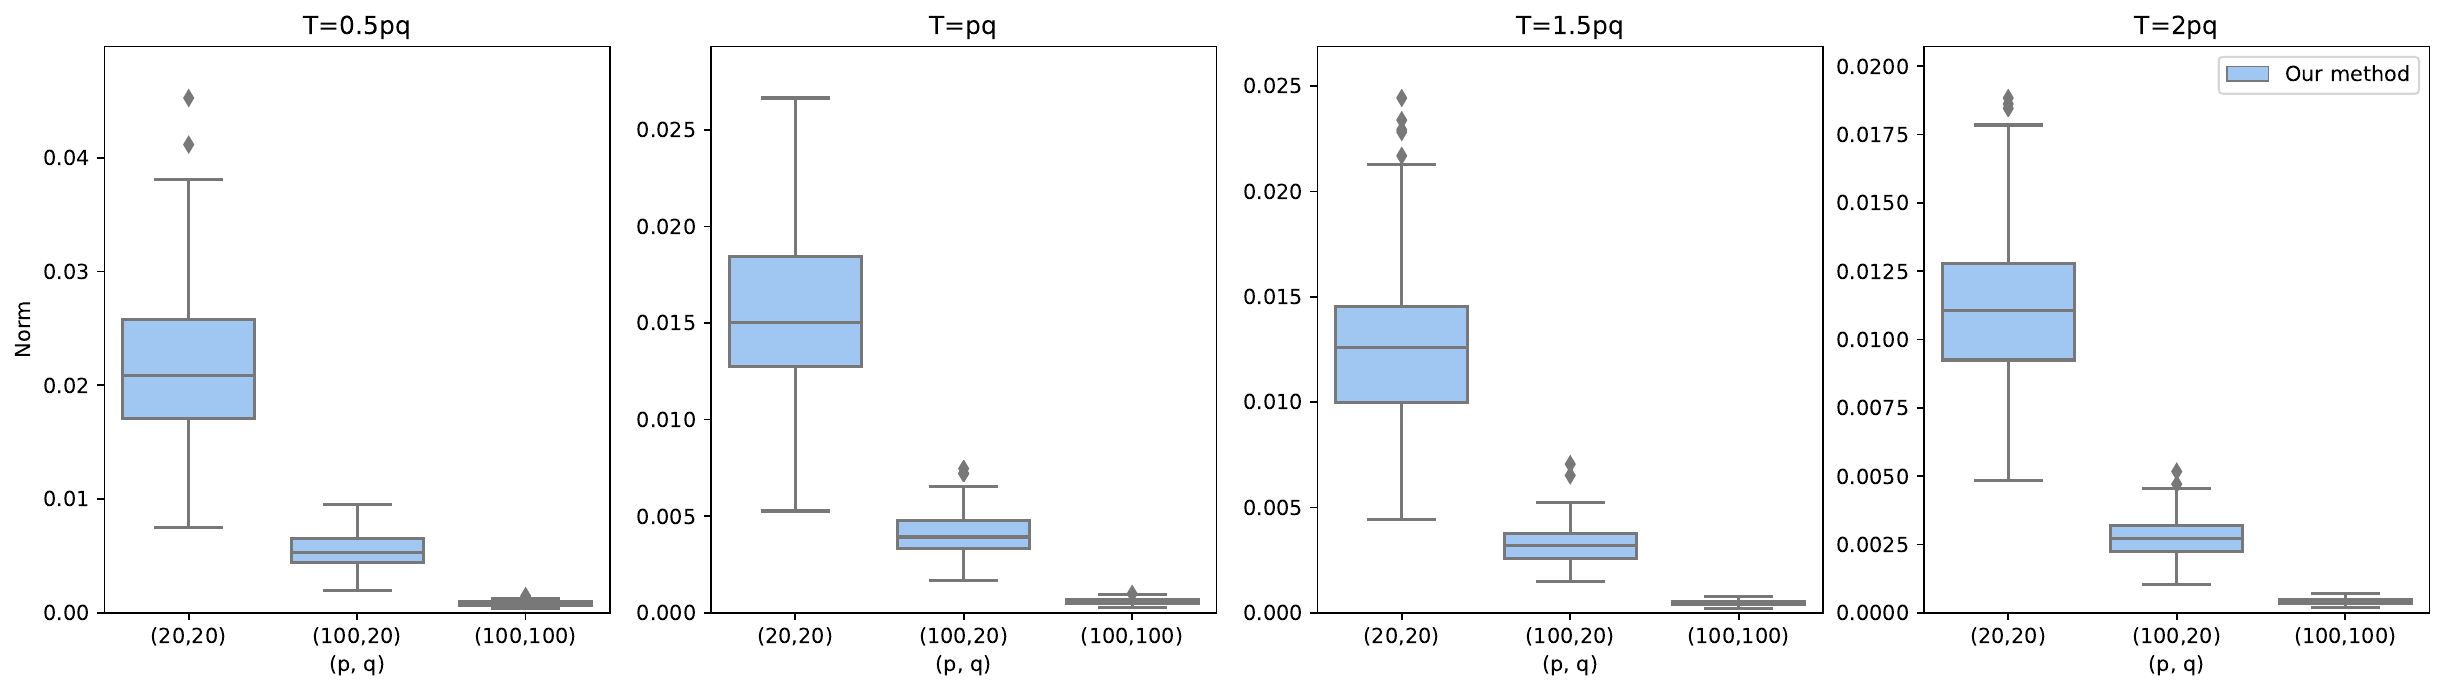}
\end{subfigure}
\caption{Boxplot of $\ell_2$ norm of distance between estimated $\hat\bF_t$ and transformed true $\bF_t$.} \label{fig:F_norm_I_III}
\end{figure}
%1D histograms with kde, corresponding QQ plots, 2D scatters of $\hat \bR - \bR\bH_R$ to show asymptotic normality

\subsection{Weakly row- or column-wisely correlated \texorpdfstring{$\bE_t$}{noise}}

This section presents results for Setting (III) where $\bE_t$ are weakly correlated cross rows and columns.
The entries of $\bF_t$ and $\bE_t$ are temporally uncorrelated, but $\bE_t$ is weakly correlated across rows and columns.
Specifically, we simulate temporally independent $\bF_t \sim \calM \calN_{3 \times 3} \left( \bzero, \bI, \bI \right)$ and $\bE_t \sim \calM \calN_{p \times q} \left( \bzero, \bU_E, \bV_E \right)$, where $\bU_E$ and $\bV_E$ both have 1's on the diagonal, while have $1/p$ and $1/q$ off-diagonal, respectively.

Table \ref{table:estim_k_III} and \ref{table:mean_sd_III} presents the frequencies of estimated $(\hat k, \hat r)$ pairs and means and standard deviations of $D(\hat{\bR}, \bR)$),$D(\hat{\bC}, \bC)$), respectively, for Setting (III).

%table estimated dimensions (Wang, Chen)
\begin{table}[htpb!]
    \centering
    \resizebox{\linewidth}{!}{
    \begin{tabular}{c| c c c c |c c c c | c c c c }
    			\multicolumn{5}{c}{$p,q = 20,20$} & \multicolumn{4}{c}{$p,q = 190,20$} & \multicolumn{4}{c}{$p,q = 100,100$}\\ \hline
    			($\hat{k},\hat{r}$)  & $T=.5pq$ & $T=pq$& $T=1.5pq$& $T=2pq$ & $T=.5pq$ & $T=pq$& $T=1.5pq$& $T=2pq$ & $T=.5pq$ & $T=pq$& $T=1.5pq$& $T=2pq$\\ \hline
    			($2,3$) & .105& .095& .1  & .08 & 0   & 0   & 0   & 0   & 0 & 0 & 0 & 0\\
                \rowcolor[HTML]{EFEFEF}  & .05 & .085 & .035 & .065 & 0 & 0 & 0 & 0 & 0 & 0 & 0 &0\\ \hline
    			($3,2$) & .08 & .095& .07 & .1  & .095& .095& .05 & .105& 0 & 0 & 0 & 0\\
                \rowcolor[HTML]{EFEFEF} & .04 & .105 & .045 & .06 &.07 & .085 & .03 & .07 & 0 &0 &0 &0\\ \hline
    			($3,3$) & .69 & .65 & .695& .685& .84 & .87 & .92 & .835& 1 & 1 & 1 & 1\\
                \rowcolor[HTML]{EFEFEF} & .84 &  .75 & .835 & .82 & .895 & .9 & .94 & .9 & 1 & 1 &1 & 1\\ \hline
    			other   & .075 & .16 & .135& .135& .065& .035  & .03& .06& 0 & 0 & 0 & 0\\
                \rowcolor[HTML]{EFEFEF} & .07 & .065 & .085 & .055 & .035 & .015 & .03 & .003 & 0 & 0 & 0 & 0\\ \hline
    	\end{tabular} }
	\caption{Table of frequencies of estimated ($\hat{k}, \hat{r}$) pairs estimated by $\alpha$-PCA (highlighted rows) and AC-PCA (not highlighted rows) under Setting (III). The truth is $(3,3)$.}  \label{table:estim_k_III}
\end{table}

\begin{figure}[htpb!]
	\centering
	\resizebox{\linewidth}{!}{\begin{tabular}{c| c c | c c | c c | c c} \hline
			& \multicolumn{2}{c}{$T = 0.5pq$} & \multicolumn{2}{c}{$T = pq$} & \multicolumn{2}{c}{$T = 1.5pq$} & \multicolumn{2}{c}{$T = 2pq$} \\ \hline
			$(p,q)$  & $\calD(\hat{\bR},\bR)$ &  $\calD(\hat{\bC},\bC)$ & $\calD(\hat{\bR},\bR)$ &  $\calD(\hat{\bC},\bC)$ & $\calD(\hat{\bR},\bR)$ &  $\calD(\hat{\bC},\bC)$ & $\calD(\hat{\bR},\bR)$ &  $\calD(\hat{\bR},\bR)$ \\ \hline
			\rowcolor[HTML]{EFEFEF}($20,20$) & .83(.38) & .84(.39)  & .81(.43) & .79(.40) & .72(.32) & .76(.39) & .74(.42) & .79(.40) \\
			& 1.41(.53) & 1.44(.51) & 1.41(.55) & 1.39(.54) & 1.30(.43) & 1.35(.41) & 1.37(.62) & 1.38(.45) \\
			\rowcolor[HTML]{EFEFEF}($100,20$) & .15(.02) & .70(.31) & .11(.01) & .74(.33) & .09(.01) & .69(.29) & .09(.02) & .67(.32) \\
			& .80(.07) & .87(.33) & .80(.07) & .91(.36) & .80(.07) & .85(.35) & .80(.07) & .85(.35) \\
			\rowcolor[HTML]{EFEFEF}($100,100$) & .06(.02) & .06(.02) & .05(.02) & .06(.02) & .05(.02) & .05(.02) & .05(.02) & .05(.02)  \\
			& .34(.02) & .34(.03) & .34(.03) & .34(.03) & .34(.03) & .34(.03) & .34(.03) & .34(.03)  \\ \hline
	\end{tabular}}
	\caption{Means and SDs in parentheses of $D(\hat{\bR}, \bR)$),$D(\hat{\bC}, \bC)$) estimated by the Chen method (highlighted) and Wang method under Setting (III). All values multiplied by 10 and rounded.} \label{table:mean_sd_III}
\end{figure}

Figure \ref{fig:space_dist_ratio_I_III} (b) shows the box plots of the space distances $\calD(\hat \bR, \bR)$, $\calD(\hat \bC, \bC)$ for both methods under Setting (III).
Note the scales of the y-axis in two sub-figures are different.
The estimation errors of $\alpha$-PCA is much smaller than AC-PCA.

Figure \ref{fig:F_norm_I_III} (b) presents the box plots of $\ell_2$ norm of distance between estimated $\hat\bF_t$ and transformed true $\bF_t$, which shows the convergence of estimated factors under Setting (III).

Figure \ref{fig:space_dist_T < sqrt(pq)} shows the box plots of the space distances $\calD(\hat \bR, \bR)$, $\calD(\hat \bC, \bC)$ for both methods under Setting (I) $T < \sqrt{pq}$ with $(p, q, T)=(100, 100, 50)$.

% boxplot space distance ratio (Wang, Chen)
\begin{figure}
    \centering
    \includegraphics[width=0.5\linewidth,keepaspectratio=true]{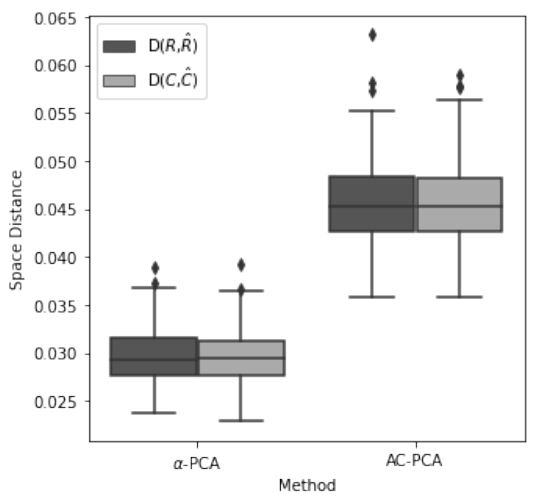}
    \caption{Box plots of the space distances of $\alpha$-PCA and AC-PCA estimators respectively. Setting I with $(p, q, T)=(100, 100, 50)$.
    The estimation errors of $\alpha$-PCA is much smaller than AC-PCA under the setting that $T < \sqrt{pq}$.}.
    \label{fig:space_dist_T < sqrt(pq)}
\end{figure}

\subsection{Asymptotic normality}

In this section, we present results of asymptotic normality for Setting (IV) with $\paran{p,q, T}$ equal to $\paran{200, 200, 100}$ and $\paran{400, 400, 250}$.
The results for asymptotic normality are based on $1000$ repetitions.
Under all settings, the presented QQ plots and histograms demonstrate the asymptotic normality expected from the theorem.

Figure \ref{fig:IV-1/3-QQ} presents the QQ plots of first dimension of the first row of $\hat\bR - \bR\bH_R$ under setting (IV) $p, q, T = 200, 200, 100$ and $ 400, 400, 250$.

Figure \ref{fig:IV-1/3-dist} presents the histograms of the first dimension of $\paran{\hat\bR_{0\cdot} - \bH_R^\top\bR_{0\cdot}}\hat\bSigma_{R_0}^{-1/2}$ with $\alpha=-1$ (left), $0$ (middle) and $1$ (right) under setting (IV) with $p, q, T = 200, 200, 150$.

Results of the other dimensions are similar.
 \begin{figure}[htpb!]
 \centering
 \begin{subfigure}{.8\textwidth}
 \caption{$p, q, T = 200, 200, 100$.}
 \centering
 \begin{subfigure}[b]{.3\linewidth}
 \centering
  \caption*{$\alpha=-1$}
 \includegraphics[width=\linewidth,keepaspectratio=true]{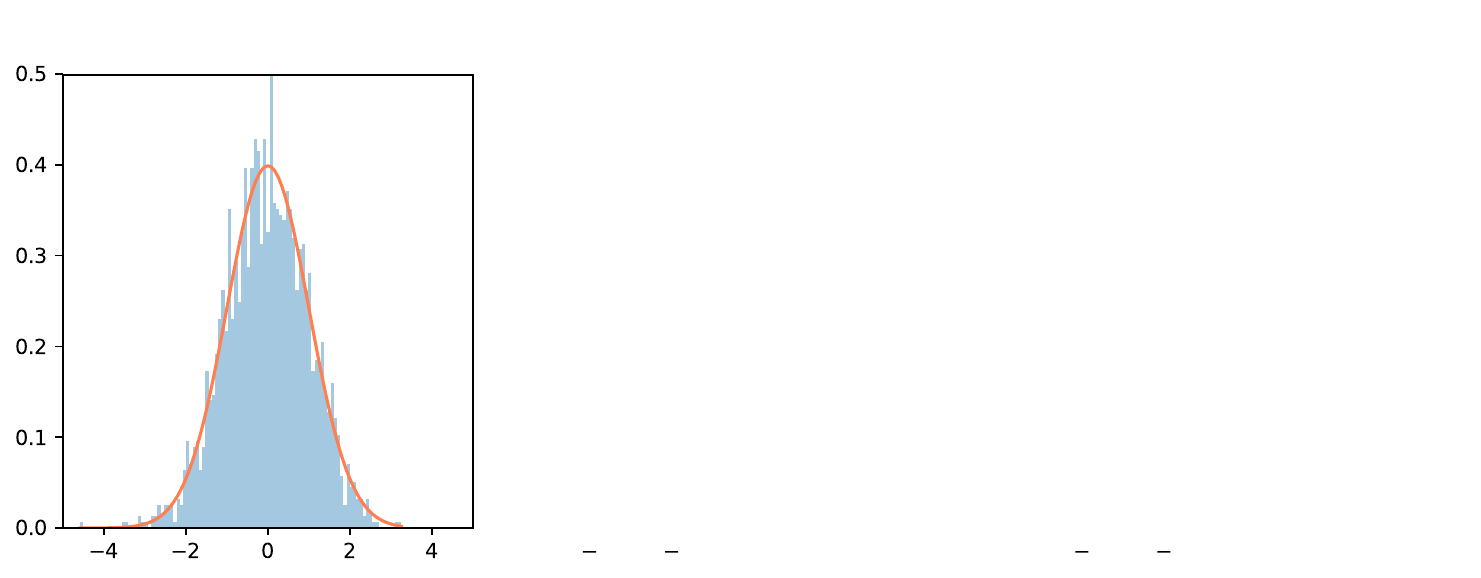}
 \end{subfigure}
 \begin{subfigure}[b]{.305\linewidth}
 \centering
 \caption*{$\alpha=0$}
 \includegraphics[width=\linewidth,keepaspectratio=true]{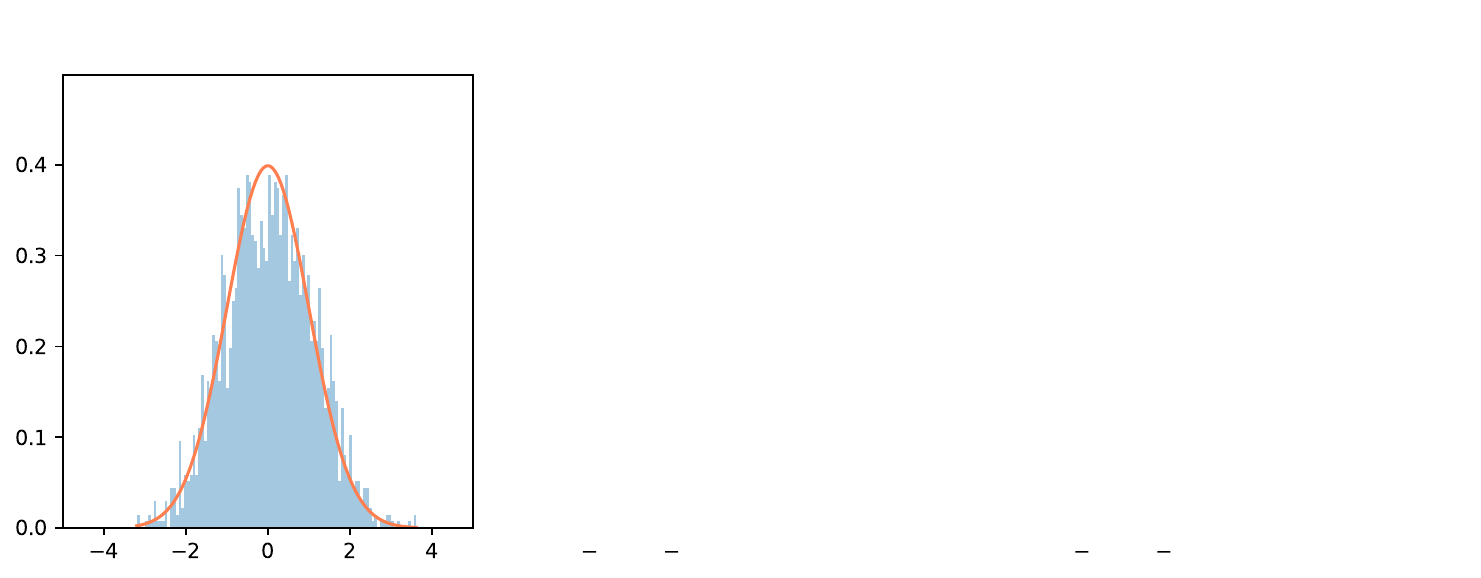}
 \end{subfigure}
 \begin{subfigure}[b]{.295\linewidth}
 \centering
 \caption*{$\alpha=1$}
 \includegraphics[width=\linewidth,keepaspectratio=true]{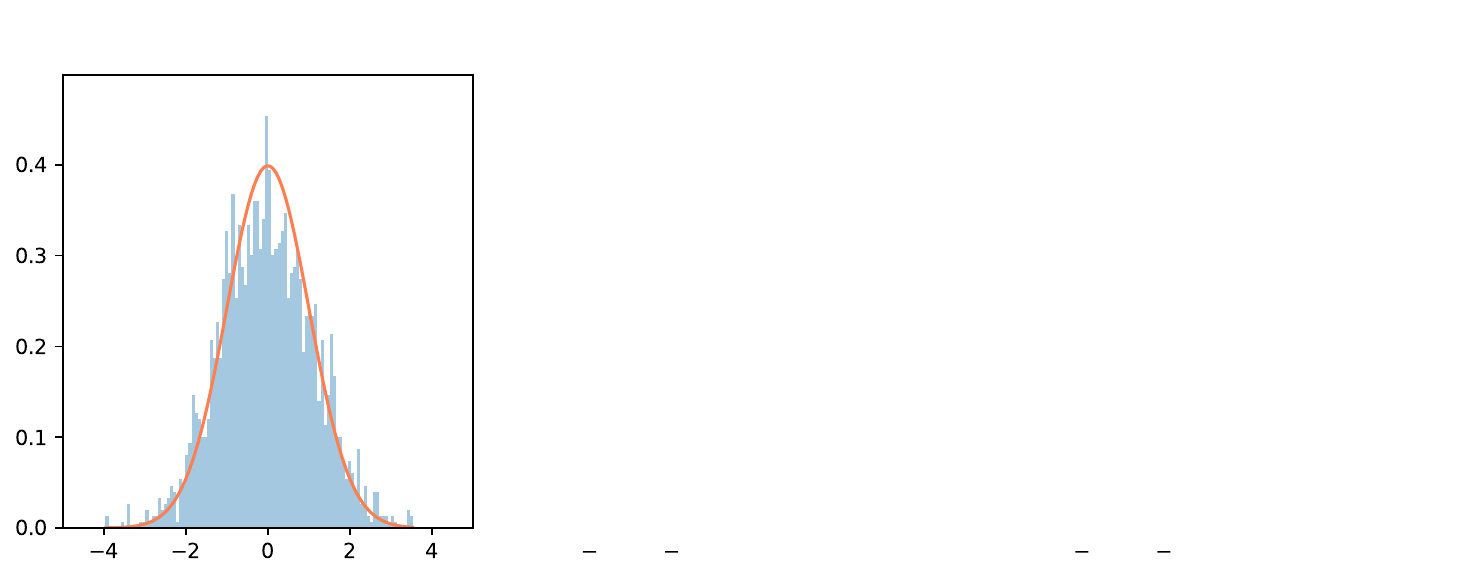}
 \end{subfigure}
 \end{subfigure}
 \begin{subfigure}{.8\textwidth}
\caption{$p, q, T = 400, 400, 250$.}
\centering
\begin{subfigure}[b]{.3\linewidth}
\centering
\caption*{$\alpha=-1$}
\includegraphics[width=\linewidth,keepaspectratio=true]{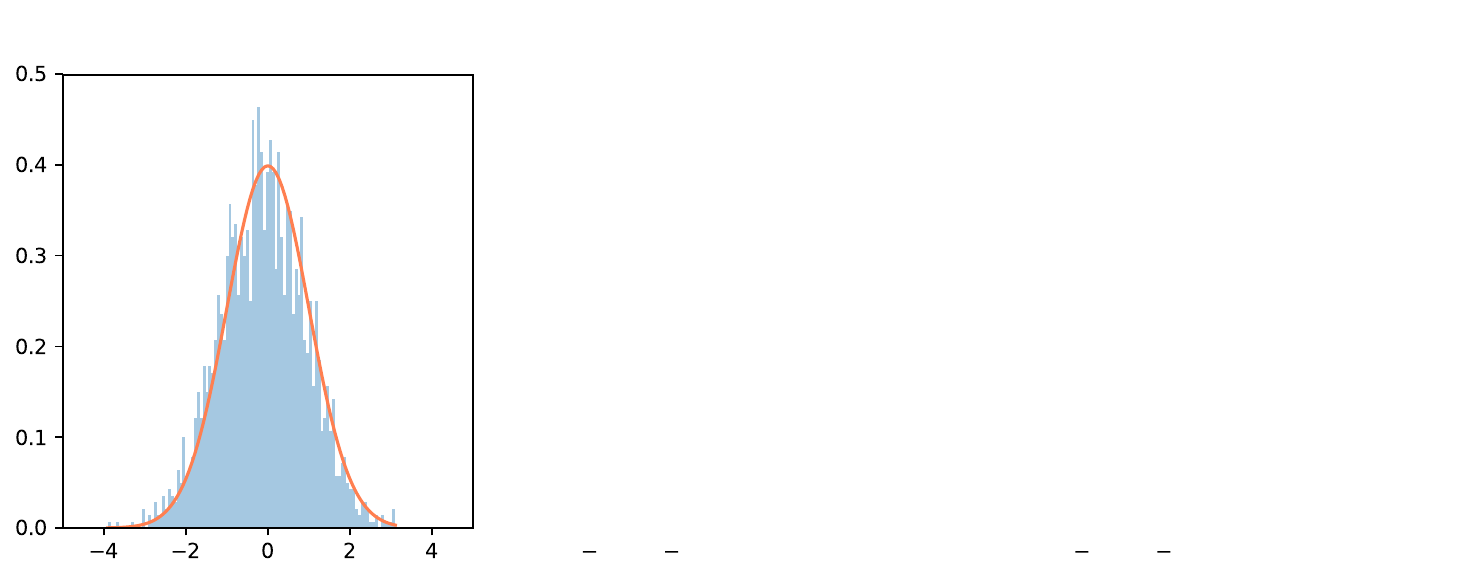}
\end{subfigure}
\begin{subfigure}[b]{.3\linewidth}
\centering
\caption*{$\alpha=0$}
\includegraphics[width=\linewidth,keepaspectratio=true]{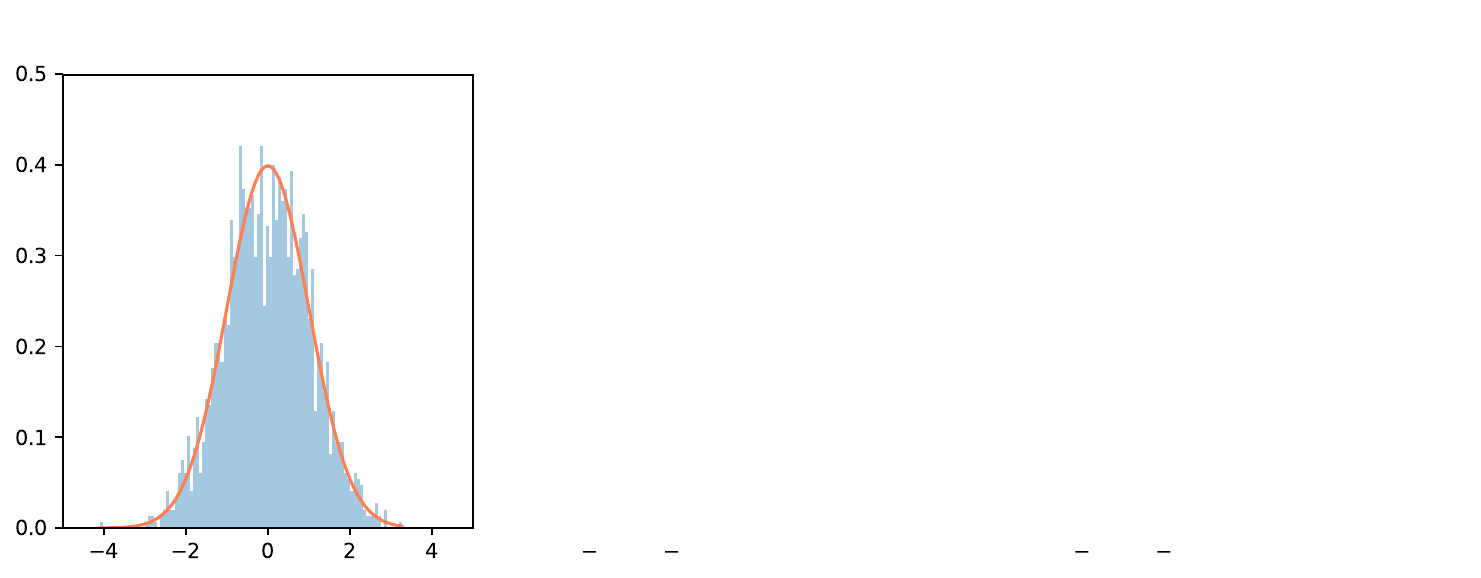}
\end{subfigure}
\begin{subfigure}[b]{.3\linewidth}
\centering
\caption*{$\alpha=1$}
\includegraphics[width=\linewidth,keepaspectratio=true]{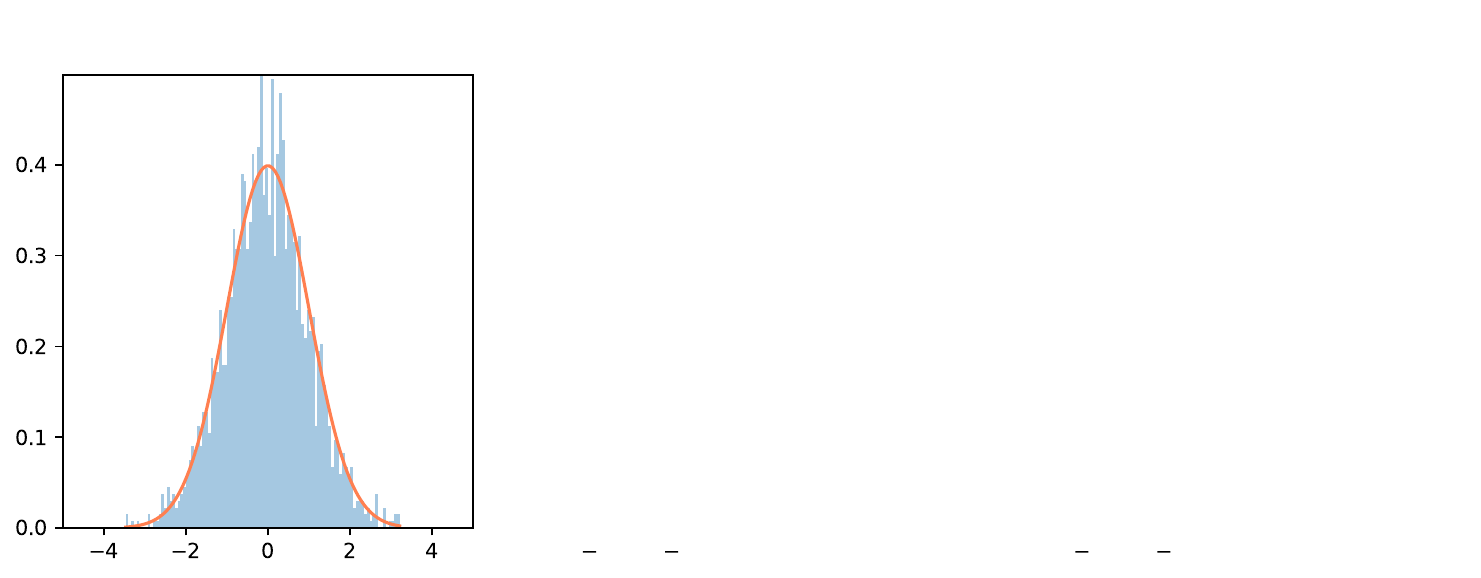}
\end{subfigure}
\end{subfigure}
\caption{Histograms of the first dimension of $\paran{\hat\bR_{0\cdot} - \bH_R^\top\bR_{0\cdot}}\hat\bSigma_{R_0}^{-1/2}$ with $\alpha=-1$ (left), $0$ (middle) and $1$ (right) under setting (IV) with $p, q, T = 200, 200, 100$ and $ 400, 400, 250$. The lines plot the distribution of standard normal distribution.}  \label{fig:IV-1/3-dist}
\end{figure}

{QQ plots of the first dimension of the first row of $\hat\bR - \bR\bH_R$ with $\alpha=-1$ (left), $0$ (middle) and $1$ (right) under setting (IV) with $p, q, T = 200, 200, 150$.}

% QQ plots
\begin{figure}[htpb!]
\centering
\begin{subfigure}[b]{0.8\textwidth}
\centering
\caption{$p, q, T = 200, 200, 100$.}
\begin{subfigure}[b]{.3\linewidth}
\centering
 \caption*{$\alpha=-1$}
\includegraphics[width=\linewidth,keepaspectratio=true]{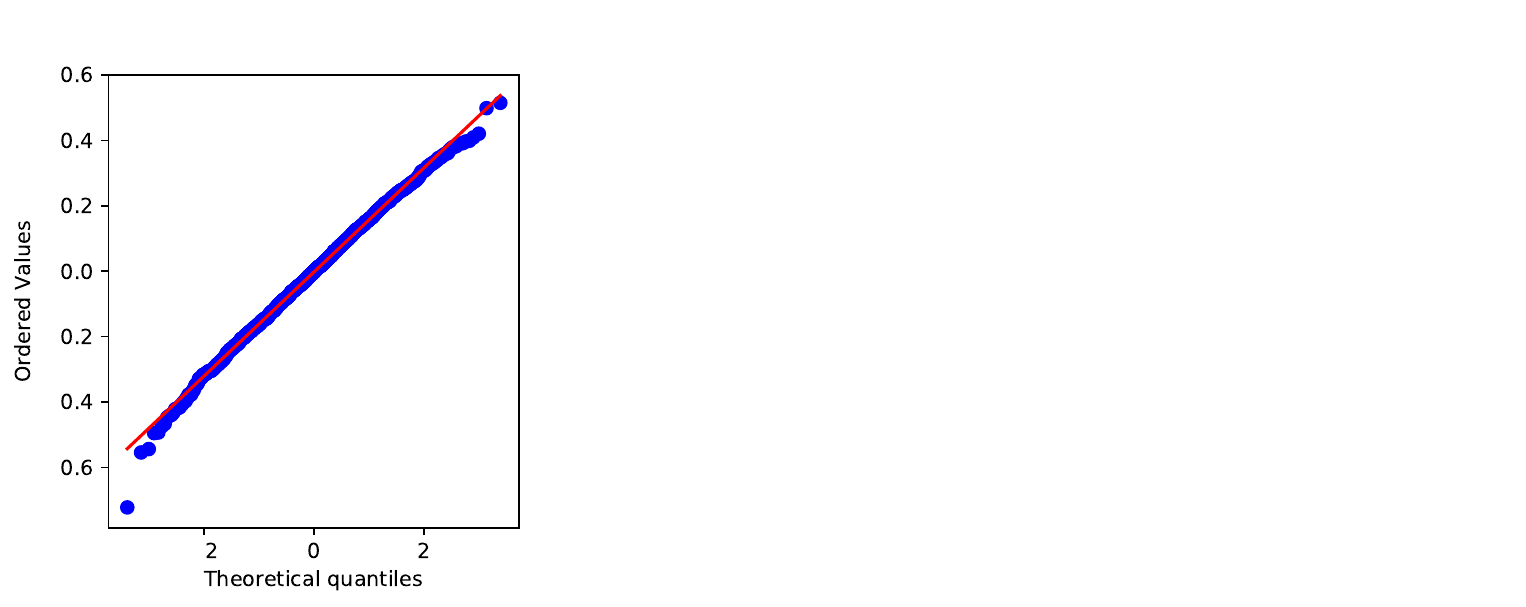}
\end{subfigure}
\begin{subfigure}[b]{.308\linewidth}
\centering
 \caption*{$\alpha=0$}
\includegraphics[width=\linewidth,keepaspectratio=true]{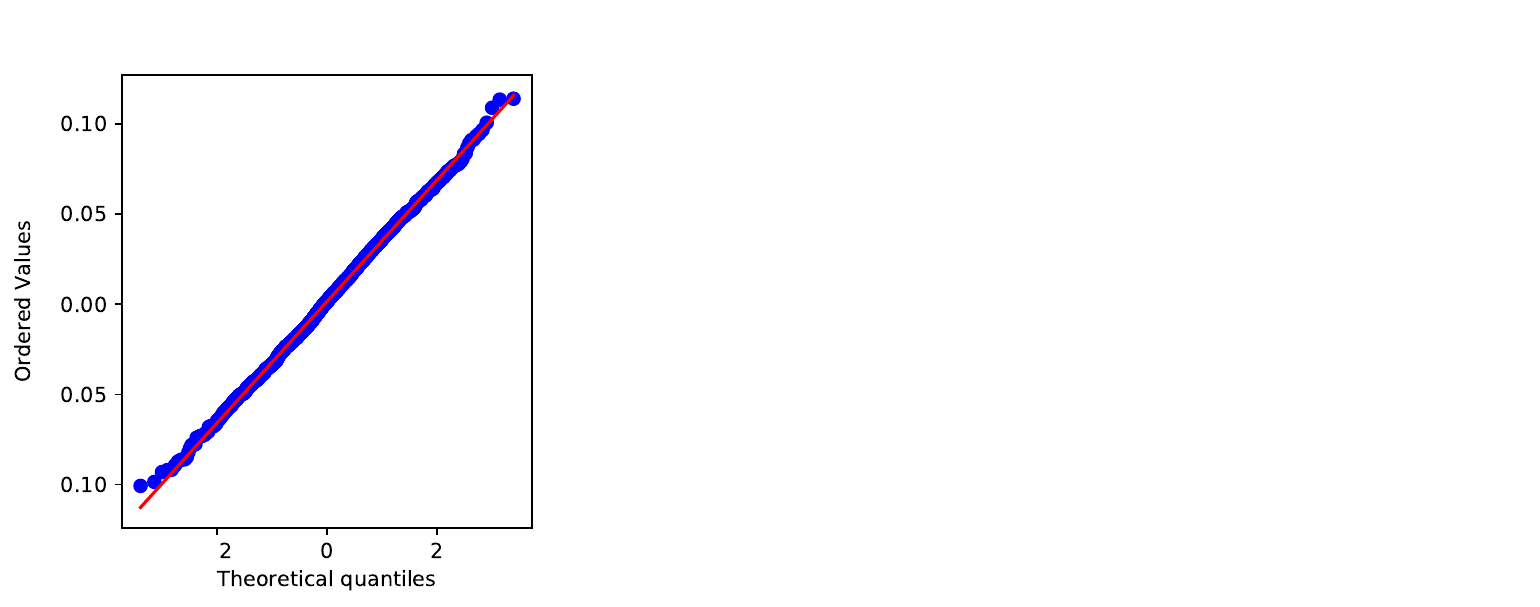}
\end{subfigure}
\begin{subfigure}[b]{.285\linewidth}
\centering
 \caption*{$\alpha=1$}
\includegraphics[width=\linewidth,keepaspectratio=true]{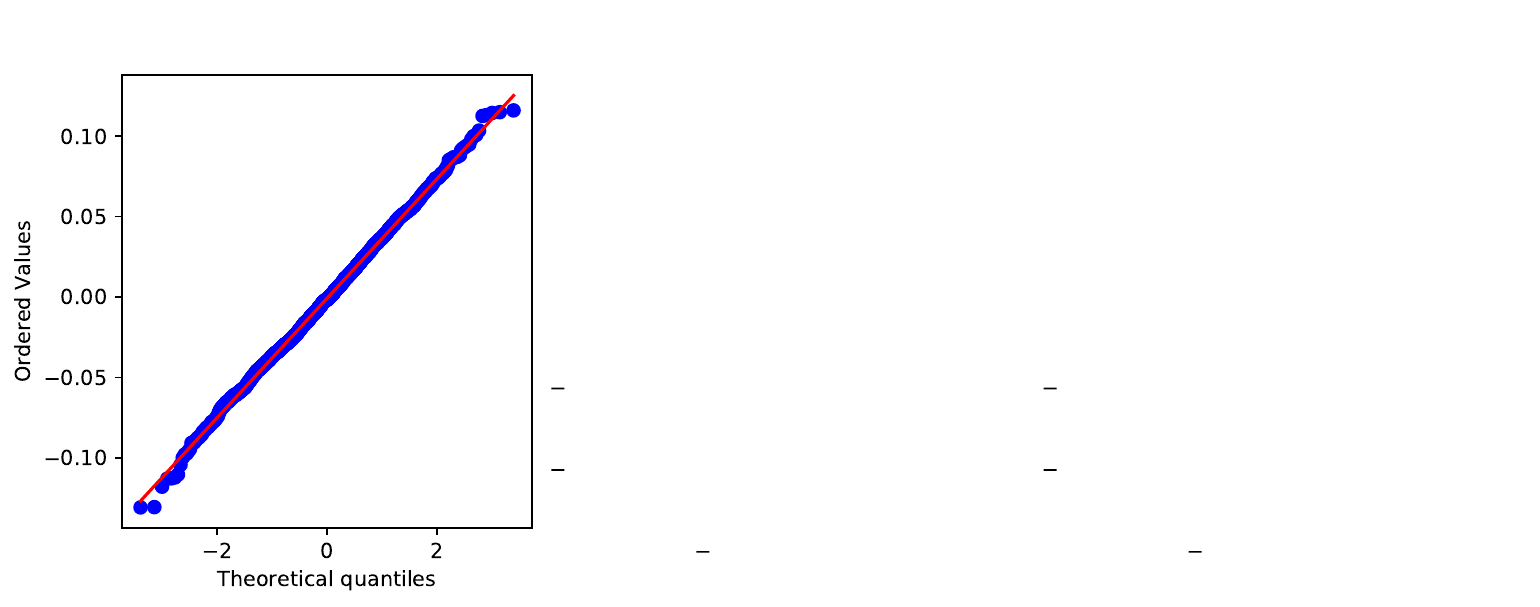}
\end{subfigure}
\end{subfigure}
\begin{subfigure}[b]{0.8\textwidth}
\centering
\caption{$p, q, T = 400, 400, 250$.}
\begin{subfigure}[b]{.29\linewidth}
\centering
 \caption*{$\alpha=-1$}
\includegraphics[width=\linewidth,keepaspectratio=true]{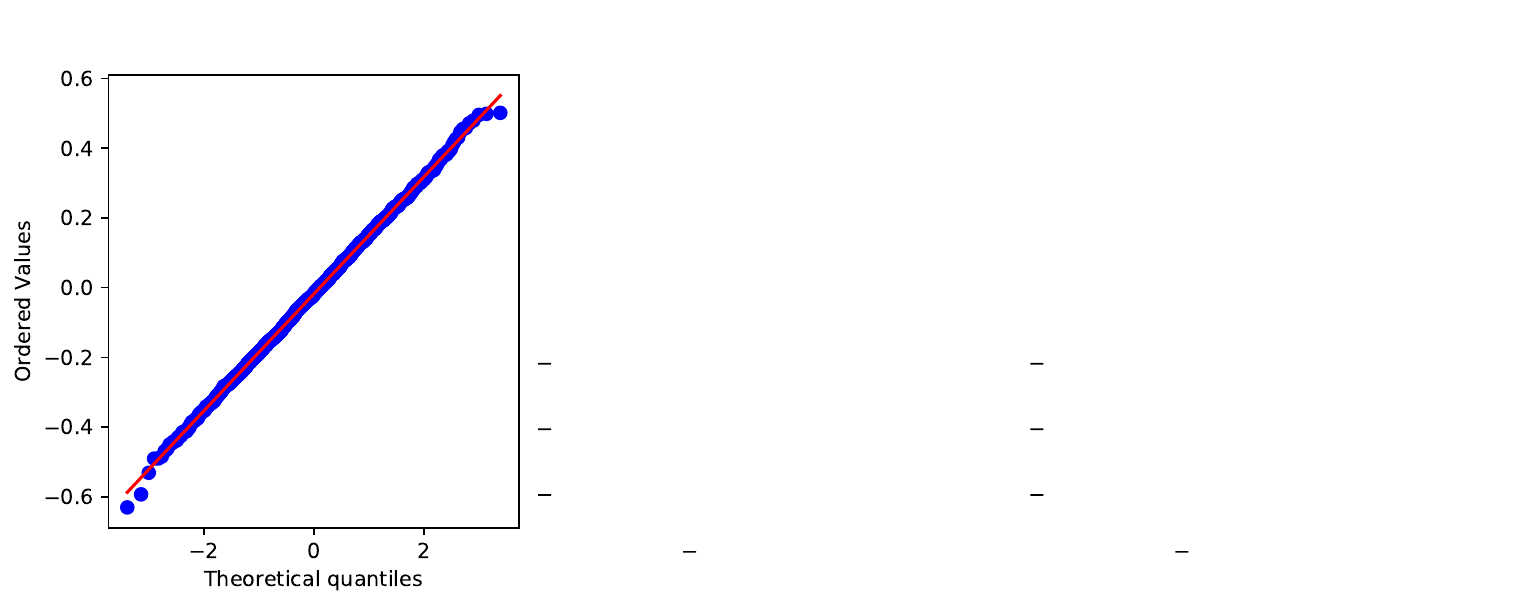}
\end{subfigure}
\begin{subfigure}[b]{.3\linewidth}
\centering
 \caption*{$\alpha=0$}
\includegraphics[width=\linewidth,keepaspectratio=true]{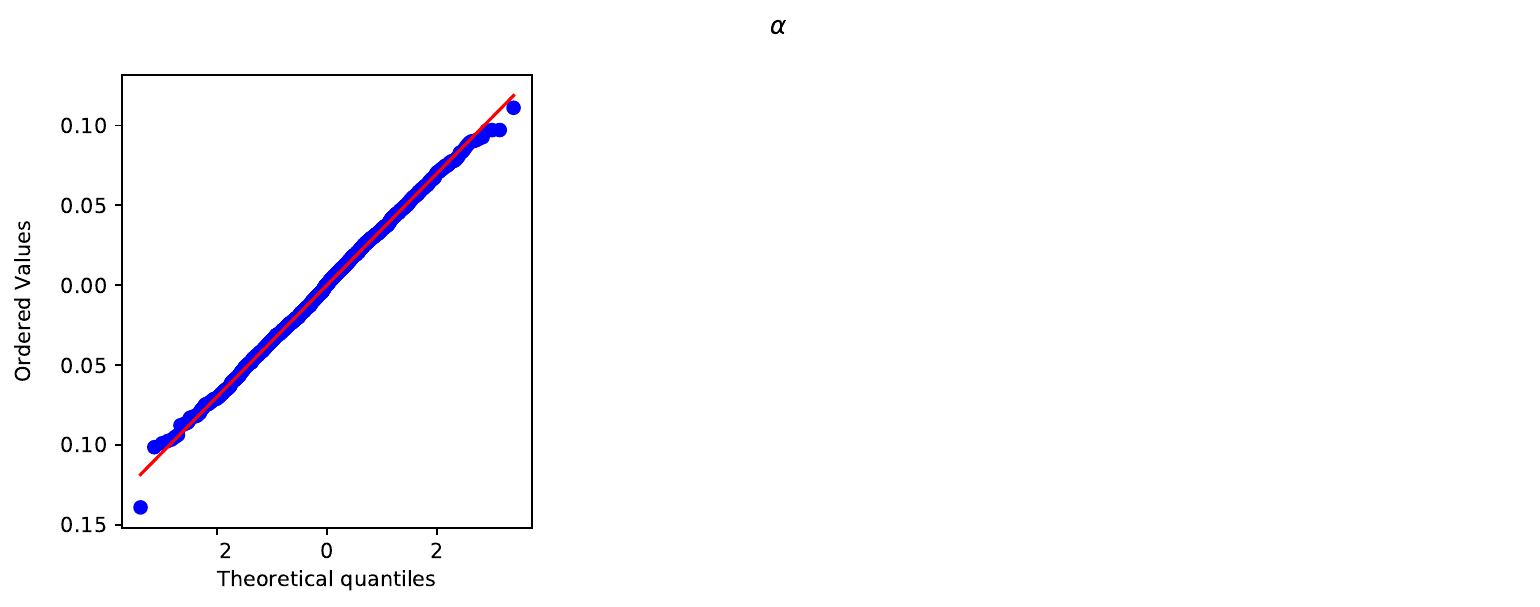}
\end{subfigure}
\begin{subfigure}[b]{.3\linewidth}
\centering
 \caption*{$\alpha=1$}
\includegraphics[width=\linewidth,keepaspectratio=true]{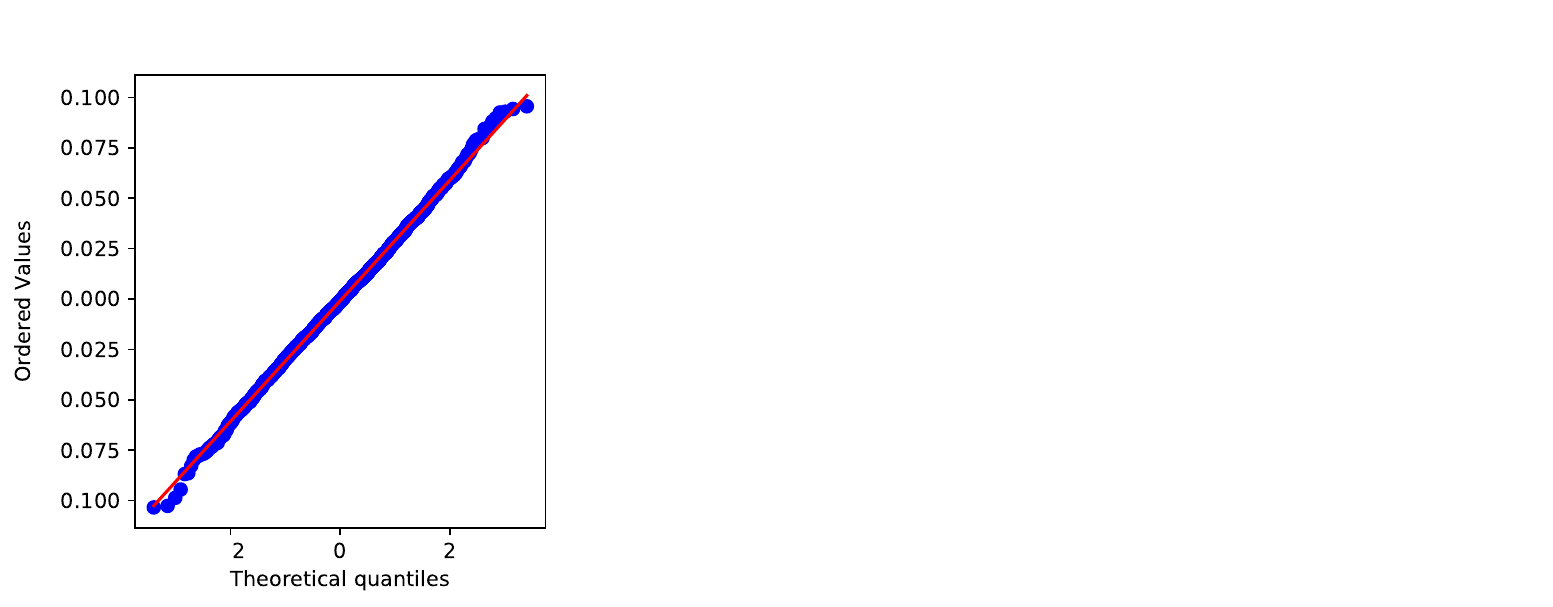}
\end{subfigure}
\end{subfigure}
\caption{QQ plots of the first dimension of the first row of $\hat\bR - \bR\bH_R$ with $\alpha=-1$ (left), $0$ (middle) and $1$ (right) under setting (IV) with $p, q, T = 200, 200, 100$ and $ 400, 400, 250$.} \label{fig:IV-1/3-QQ}
\end{figure}
