# Supplementary material for: Statistical Inference for High-Dimensional Matrix-Variate Factor Model
Source: arXiv:2001.01890 source file (2022-10-19)
Supplement: Supplementary file 2 [file data-appendix.tex]

\section{Multinational Macroeconomic Indexes Dataset} \label{appendix:cross_country_macro_dataset}

Table \ref{table:macro_index_data} lists the short name of each series, its mnemonic (the series label used in the OECD database), the transformation applied to the series, and a brief data description. All series are from the OECD Database. In the transformation column, $\Delta$ denote the first difference, $\Delta\ln$ denote the first difference of the logarithm. GP denotes the measure of growth rate last period.

\begin{table}[H]
\centering
\resizebox{\textwidth}{!}{%
\begin{tabular}{lccc}
\hline
Short name & Mnemonic & Tran & description\\
\hline
CPI: Food & CPGDFD & $\Delta^2 \ln$ & Consumer Price Index: Food, seasonally adjusted \tabularnewline
\hline
CPI: Ener & CPGREN & $\Delta^2 \ln$ & Consumer Price Index: Energy, seasonally adjusted \tabularnewline
\hline
CPI: Tot & CPALTT01 & $\Delta^2 \ln$ & Consumer Price Index:  Total, seasonally adjusted \\
\hline
IR: Long & IRLT & $\Delta$ & Interest Rates: Long-term gov bond yields\\
\hline
IR: 3-Mon & IR3TIB & $\Delta$ & Interest Rates: 3-month Interbank rates and yields\\
\hline
P: TIEC & PRINTO01 & $\Delta \ln$ & Production: Total industry excl
construction \\
\hline
P: TM  & PRMNTO01 & $\Delta \ln$ & Production: Total manufacturing \\
\hline
GDP  & LQRSGPOR & $\Delta \ln$ & GDP: Original (Index 2010 = 1.00, seasonally adjusted) \\
\hline
IT: Ex & XTEXVA01 & $\Delta \ln$ & International Trade: Total Exports Value (goods) \\
\hline
IT: Im & XTIMVA01 & $\Delta \ln$ & International Trade: Total Imports Value (goods) \\
\hline
\end{tabular}
} %
\caption{Data transformations, and variable definitions}
\label{table:macro_index_data}
\end{table}

\begin{table}[H]
\centering
\scalebox{1}{
\begin{tabular}{lc||lc}
\hline
\multicolumn{1}{c}{Country} & ISO ALPHA-3 Code & \multicolumn{1}{c}{Country} & ISO ALPHA-3 Code \\ \hline
United States of America & USA & United Kingdom & GBR \\
Canada & CAN & Finland & FIN \\
New Zealand & NZL & Sweden & SWE \\
Australia & AUS & France & FRA \\
Norway & NOR & Netherlands & NLD \\
Ireland & IRL & Austria & AUT \\
Denmark & DNK & Germany & DEU \\ \hline
\end{tabular}}
\caption{Countries and ISO Alpha-3 Codes in Macroeconomic Indices Application}
\label{table:oecd_country_sel}
\end{table}

Figure \ref{fig:oecd_mts_plot} in the supplemental material shows the transformed time series of macroeconomic indicators of multiple countries.
It is obvious that there exist some similar patterns among time series in the same row or column.

\begin{figure}[ht!]
    \centering
    \includegraphics[width=0.8\linewidth,,keepaspectratio=true]{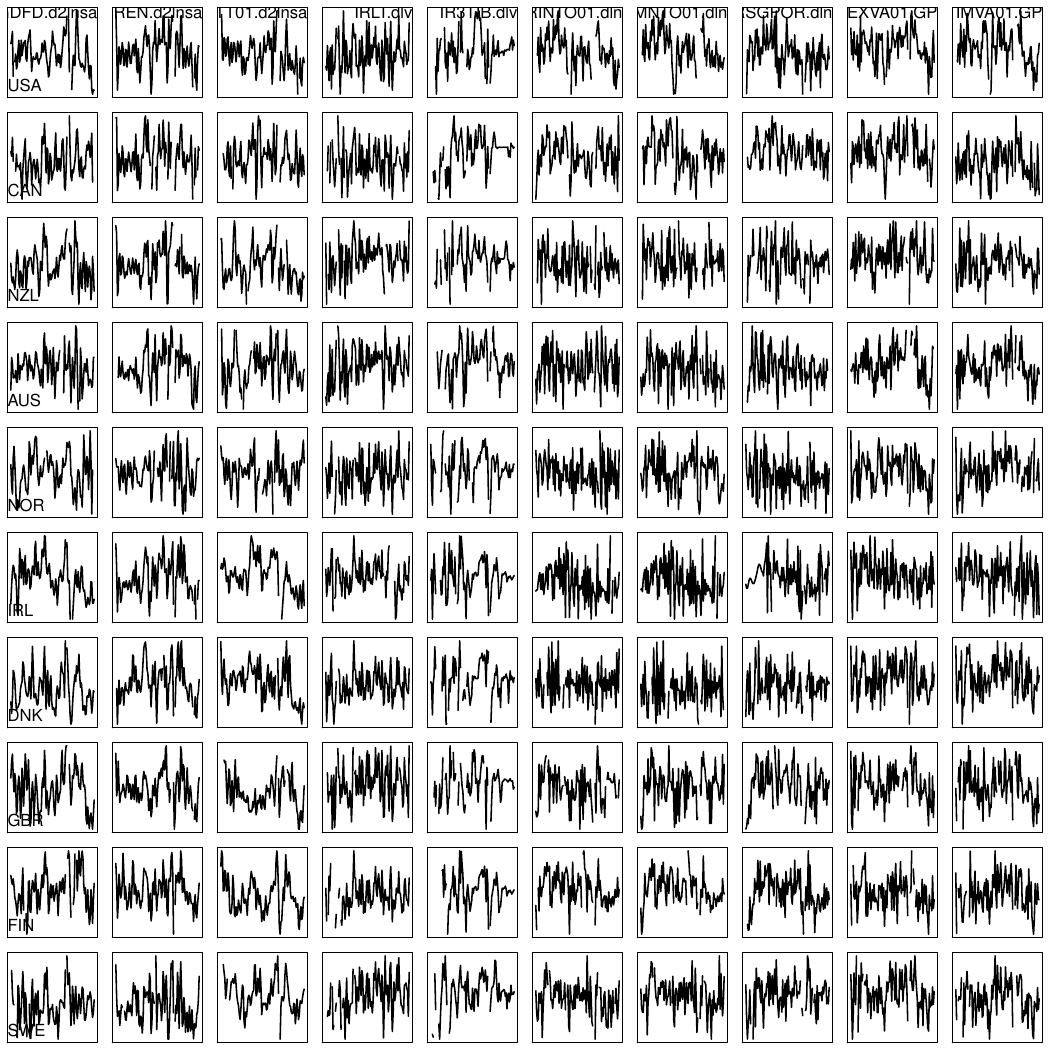}
    \caption{Time series plots of macroeconomic indicators of multiple countries (after data transformation). Only a subset of the countries and indicators is plotted due to the space limit.}
    \label{fig:oecd_mts_plot}
\end{figure}

\section{More results on the image datasets} \label{appendix:image}

\begin{figure}[ht!]
    \centering
    \begin{subfigure}[b]{0.8\textwidth}
        \centering
        \includegraphics[width=\linewidth,height=\textheight,keepaspectratio=true]{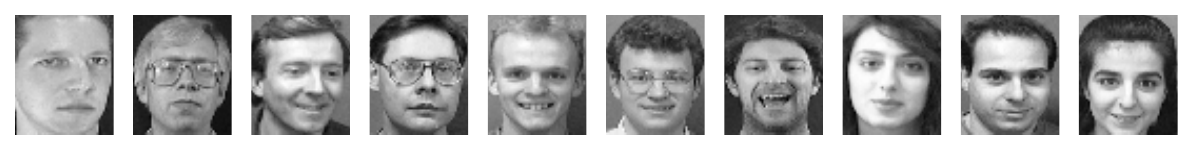}
    \end{subfigure}
    \begin{subfigure}[b]{0.8\textwidth}
        \centering
        \includegraphics[width=\linewidth,height=\textheight,keepaspectratio=true]{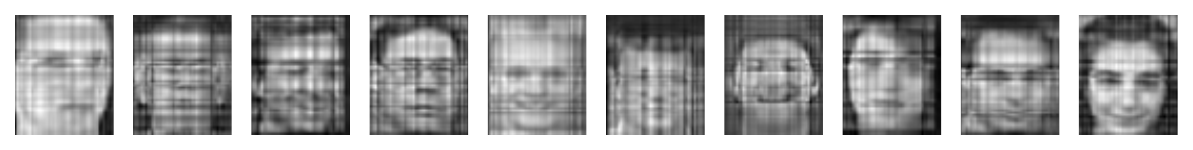}
    \end{subfigure}
    \begin{subfigure}[b]{0.8\textwidth}
        \centering
        \includegraphics[width=\linewidth,height=\textheight,keepaspectratio=true]{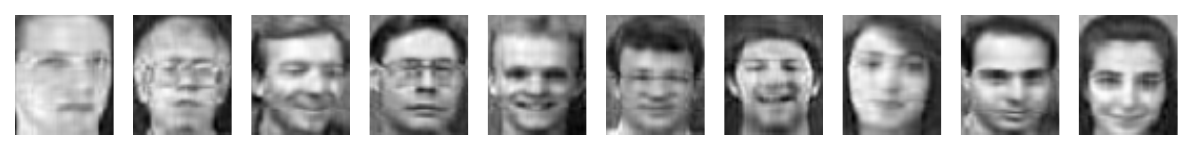}
    \end{subfigure}
    \begin{subfigure}[b]{0.8\textwidth}
        \centering
        \includegraphics[width=\linewidth,height=\textheight,keepaspectratio=true]{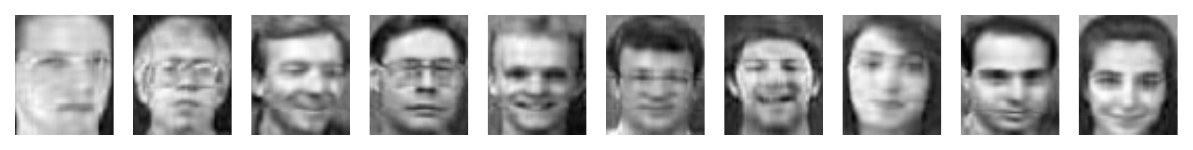}
    \end{subfigure}
    \begin{subfigure}[b]{0.8\textwidth}
        \centering
        \includegraphics[width=\linewidth,height=\textheight,keepaspectratio=true]{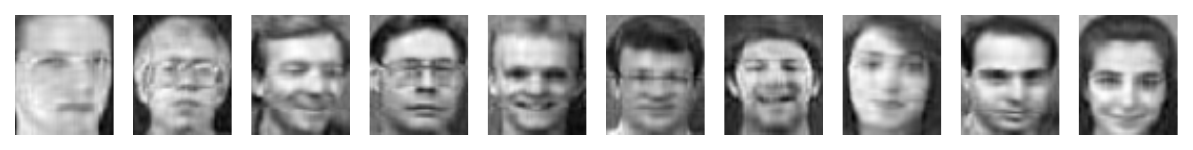}
    \end{subfigure}
    \caption{ORL face reconstruction with $15 \times 15$ latent dimension. The 1-st row displays ten raw images from ORL data set. The 2nd to the 5th row correspond to reconstruction using our method with $\alpha = -1$, $0$, $1$ and $2$, respectively.
        The compression ratio is approximately 2.18\%.  %{\bf Q: don't know how compress ration is computed}
    }
    \label{fig:orl-faces}
\end{figure}

\begin{figure}[ht!]
    \centering
    \begin{subfigure}[b]{0.8\textwidth}
        \centering
        \includegraphics[width=\linewidth,height=\textheight,keepaspectratio=true]{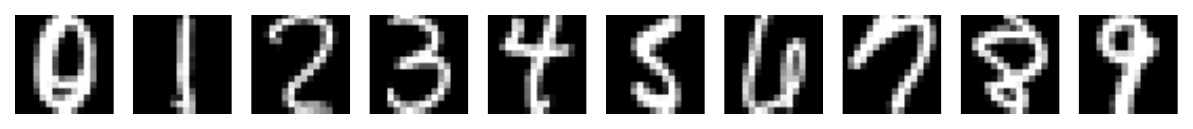}
    \end{subfigure}
    \begin{subfigure}[b]{0.8\textwidth}
        \centering
        \includegraphics[width=\linewidth,height=\textheight,keepaspectratio=true]{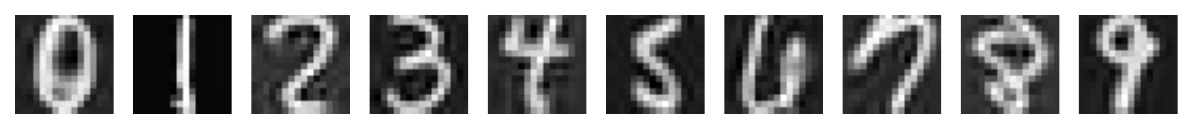}
    \end{subfigure}
    \begin{subfigure}[b]{0.8\textwidth}
        \centering
        \includegraphics[width=\linewidth,height=\textheight,keepaspectratio=true]{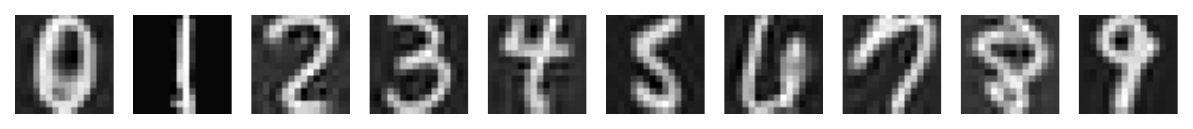}
    \end{subfigure}
    \begin{subfigure}[b]{0.8\textwidth}
        \centering
        \includegraphics[width=\linewidth,height=\textheight,keepaspectratio=true]{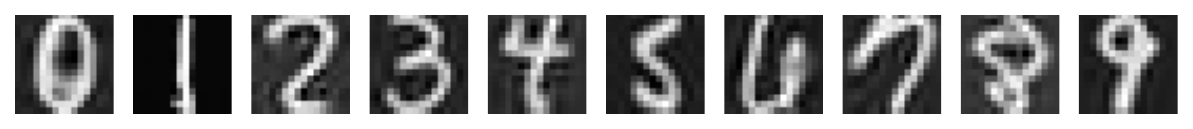}
    \end{subfigure}
    \begin{subfigure}[b]{0.8\textwidth}
        \centering
        \includegraphics[width=\linewidth,height=\textheight,keepaspectratio=true]{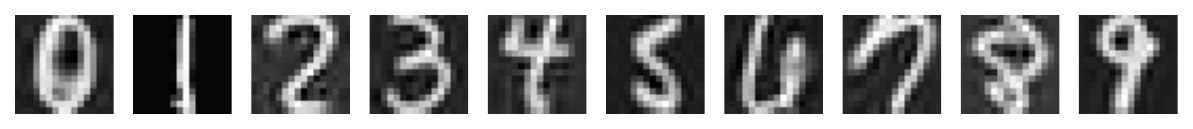}
    \end{subfigure}
    \caption{USPS digits reconstruction  with $9 \times 9$ latent dimension.
        The compression ratio is approximately 31.64\%.
        The 1-st row displays ten raw images from USPS data set. The 2nd to the 5th row correspond to reconstruction using our method with $\alpha = -1$, $0$, $1$ and $2$, respectively.}
    \label{fig:usps-digits}
\end{figure}

\section{Codes}

All codes are available online in \url{https://github.com/ElynnCC/Matrix-Factor-Models}.
